# Supplementary material for: Indirect optical manipulation of the antiferromagnetic order of insulating NiO by ultrafast interfacial energy transfer
Source: arXiv:2205.02686 source file (2026-11-06)
Supplement: Supplementary file 1 [file Supplement_arxiv.tex]

\documentclass[aps,prl,preprintnumbers,amsmath,amssymb,notitlepage,superscriptaddress]{revtex4}
\pdfoutput=1
%\usepackage[dvips]{epsfig}
%\usepackage{subfigure}
% For displaying figures
\usepackage{graphicx} 
\usepackage{floatrow}
\usepackage{subfig}
\usepackage{caption}
\floatsetup[figure]{style=plain,subcapbesideposition=top}
%\usepackage{longtable}
% Provides special text symbols
\usepackage{textcomp} 
%\usepackage[T1]{fontenc}
% Provides us with Umlaute
\usepackage[utf8]{inputenc}
%\usepackage{tikz}
%\usepackage{ulem}
%Provides colors
\usepackage{xcolor}
% For handling pdf
\usepackage[final]{pdfpages}
%\newcommand{\revtex}{REV\TeX\ }
%\newcommand{\classoption}[1]{\texttt{#1}}
%\newcommand{\macro}[1]{\texttt{\textbackslash#1}}
%\newcommand{\m}[1]{\macro{#1}}
%\newcommand{\env}[1]{\texttt{#1}}
%\setlength{\textheight}{9.5in}
%\newcommand{\unit}[1]{\ensuremath{\, \mathrm{#1}}}
%\raggedbottom
\usepackage{float}
\usepackage{miller}

\usepackage{hyperref}
\usepackage{siunitx}
\usepackage{physics}

\begin{document}

\newcommand{\gpi}{\textrm{\greektext p}}
\newcommand{\gmu}{\textrm{\greektext m}}
\newcommand{\beginsupplement}{%
        \setcounter{table}{0}
        \renewcommand{\thetable}{S\arabic{table}}%
        \setcounter{figure}{0}
        \renewcommand{\thefigure}{S\arabic{figure}}%
        \renewcommand{\theequation}{S\arabic{equation}}
    }

\newcommand{\highl}[1]{{\color{red}#1}}
\newcommand{\commnt}[1]{{\it \color{blue}#1}}

    \title{Indirect optical manipulation of the antiferromagnetic order of insulating NiO by ultrafast interfacial energy transfer}
    
    \author{Stephan~\surname{Wust}}
    \email{wust@rhrk.uni-kl.de}
    	\affiliation{Department of Physics and Research Center OPTIMAS, Technische Universit{\"a}t Kaiserslautern, 67663 Kaiserslautern, Germany}
    
    \author{Christopher~\surname{Seibel}}
    	\affiliation{Department of Physics and Research Center OPTIMAS, Technische Universit{\"a}t Kaiserslautern, 67663 Kaiserslautern, Germany}
    
    \author{Hendrik~\surname{Meer}}
    	\affiliation{Institute of Physics, Johannes Gutenberg-University Mainz, 55099 Mainz, Germany}
    
    \author{Paul~\surname{Herrgen}}
    	\affiliation{Department of Physics and Research Center OPTIMAS, Technische Universit{\"a}t Kaiserslautern, 67663 Kaiserslautern, Germany}
    
    \author{Christin~\surname{Schmitt}}
    	\affiliation{Institute of Physics, Johannes Gutenberg-University Mainz, 55099 Mainz, Germany}
    
    \author{Lorenzo~\surname{Baldrati}}
    	\affiliation{Institute of Physics, Johannes Gutenberg-University Mainz, 55099 Mainz, Germany}
    
    \author{Rafael~\surname{Ramos}}
    	\affiliation{CIQUS, Departamento de Qu\'imica-F\'isica, Universidade de Santiago de Compostela, Santiago de Compostela, Spain}
    	\affiliation{WPI Advanced Institute for Materials Research, Tohoku University, Sendai 980-8577, Japan}
    
	\author{Takashi Kikkawa}
		\affiliation{Department of Applied Physics, The University of Tokyo, Tokyo 113-8656, Japan}
    
    \author{Eiji Saitoh}
		\affiliation{Department of Applied Physics, The University of Tokyo, Tokyo 113-8656, Japan}
		\affiliation{Institute for AI and Beyond, The University of Tokyo, Tokyo 113-8656, Japan}
		\affiliation{WPI Advanced Institute for Materials Research, Tohoku University, Sendai 980-8577, Japan}
		\affiliation{Advanced Science Research Center, Japan Atomic Energy Agency, Tokai 319-1195, Japan}
    
	\author{Olena~\surname{Gomonay}}
		\affiliation{Institute of Physics, Johannes Gutenberg-University Mainz, 55099 Mainz, Germany}
		
	\author{Jairo~\surname{Sinova}}
		\affiliation{Institute of Physics, Johannes Gutenberg-University Mainz, 55099 Mainz, Germany}
		\affiliation{Institute of Physics, Czech Academy of Sciences, Cukrovarnick\'a 10, 162 00 Praha 6, Czech Republic}
		
	\author{Yuriy~\surname{Mokrousov}}
		\affiliation{Institute of Physics, Johannes Gutenberg-University Mainz, 55099 Mainz, Germany}
		\affiliation{Peter Gr\"unberg Institut and Institute for Advanced Simulation, Forschungszentrum J\"ulich and JARA, 52425 J\"ulich, Germany.}
		
    \author{Hans~Christian~\surname{Schneider}}
    	\affiliation{Department of Physics and Research Center OPTIMAS, Technische Universit{\"a}t Kaiserslautern, 67663 Kaiserslautern, Germany}
    	
    \author{Mathias~\surname{Kl\"aui}}
    	\affiliation{Institute of Physics, Johannes Gutenberg-University Mainz, 55099 Mainz, Germany}
    	
    \author{Baerbel~\surname{Rethfeld}}
    	\affiliation{Department of Physics and Research Center OPTIMAS, Technische Universit{\"a}t Kaiserslautern, 67663 Kaiserslautern, Germany}
    	
    \author{Benjamin~\surname{Stadtm\"uller}}
    	\email{bstadtmueller@physik.uni-kl.de}
    	\affiliation{Department of Physics and Research Center OPTIMAS, Technische Universit{\"a}t Kaiserslautern, 67663 Kaiserslautern, Germany}
    	\affiliation{Institute of Physics, Johannes Gutenberg-University Mainz, 55099 Mainz, Germany}
    \author{Martin~\surname{Aeschlimann}}
    	\affiliation{Department of Physics and Research Center OPTIMAS, Technische Universit{\"a}t Kaiserslautern, 67663 Kaiserslautern, Germany}
    \date{\today}

\maketitle
\beginsupplement

\section{Magneto-optical birefringence}
\label{mob}
The magnetic order of the antiferromagnet NiO is monitored by its magneto-optical birefringence (MOBF). Below its Néel-temperature, NiO exhibits a rhombohedral distortion, which shows a uniaxial anisotropy in reflectivity \cite{Germann1974}. Depending on the relative angle of this anisotropy axis to the linear polarization of the incoming light, this causes a rotation of polarization upon reflection on the sample~\cite{Xu2019a}. 

\begin{equation}
\label{eq:mobf}
    \theta_{pol} = \frac{r_{\parallel}-r_{\perp}}{r_{\parallel}+r_{\perp}} \sin{2\varphi}
\end{equation}

In this equation, $r_{\parallel}$ and $r_{\perp}$ are the reflection coefficients parallel and perpendicular to the in-plane projection of the distortion $\vec{T}_{D}^{\parallel}$, $\varphi$ is the relative angle between the polarization of the incoming light and $\vec{T}_{D}^{\parallel}$, and $\theta_{pol}$ represents the resulting rotation of the polarization of the reflected probe beam \cite{Xu2019a}. This anisotropy axis is identified by rotating the sample by 360°. A sketch explaining the measurement geometry and the corresponding calibration curve are shown in Figs. \ref{fig:calibration}(a) and (b).

In our time-resolved (pump-probe) experiment, we record the birefringence signal for two sample angles with antisymmetric MOBF contribution. This allows us to obtain a pure MOBF signal without pure optical contribution by subtracting these two experimental signals from each other. This procedure is well established for time-resolved Kerr studies of ferromagnetic materials.

\section{Experimental details}
\label{exp}

Our time-resolved experiments were performed with an all-optical pump-probe setup using an amplified
Ti:Sapphire laser system (1.55$\,$eV, 35$\,$fs, 1$\,$kHz, 7$\,$mJ per pulse) to generate the pump and probe beams. We determined the temporal pulse length at the sample position to 40$\,\pm\,$3$\,$fs for the 1.55$\,$eV pump pulse and 47$\,\pm\,$5$\,$fs for the 3.1$\,$eV probe pulse by employing auto- and cross-correlation methods. The probe was created by second-harmonic generation of the fundamental laser radiation with a Beta-Barium-Borate (BBO) crystal. Both s-polarized pulses were focused on the sample under normal incidence (Angle relative to sample normal $<$ 1$\,^{\circ}$). Both beams were adjusted to the rotational center of the sample, to ensure probing and pumping the same sample position independent of the sample angle $\varphi$. The laser spot sizes used in our experiment are shown in the following section.

\begin{figure}[H]
\centering
\includegraphics[width=\textwidth]{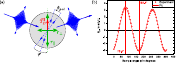}
\caption{(a) Detailed sketch explaining the measurement of the magneto-optical birefringence with an illustration of the variables shown in equation (\ref{eq:mobf}). (b) Magneto-optical birefringence signal in dependency of the sample angle $\varphi$. Markings indicate the angles chosen for the time-resolved measurements.}
\label{fig:calibration}
\end{figure}

\section{Determining the applied fluence}

For the applied pump fluences presented in the main manuscript, the spot size of the pump beam was determined with a CCD camera (see \ref{fig:spots}). The intensity profile of the resulting image was fitted by a two-dimensional Gaussian resulting in the $1/e^{2}$-width of both beams. The size of the probe spot was chosen to be smaller than the pump spot.

\begin{figure}[H]
\centering
\includegraphics[width=\textwidth]{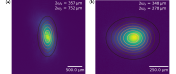}
\caption{Spot images of focused a) pump and b) probe beam. Images were fitted by a 2d-Gaussian function to determine the $1/e^{2}$ radii in x- and y-direction.}
\label{fig:spots}
\end{figure}

The total applied peak fluence was then determined using the following definition:

\begin{equation}
    \Phi = \frac{2P}{f \pi w_{x} w_{y}}
\end{equation}

Here $P$ represents the applied laser power, $f$ is the repetition rate of the laser while $w_{x}$ and $w_{y}$ are the corresponding $1/e^{2}$ spot-radii in x- and y-direction determined in Fig. \ref{fig:spots} \cite{gort2020ultrafast}.

\newpage

\section{Identification of magnon modes}
\label{magnon}

Here, we discuss the quantification of the frequency of the coherent magnon mode observed in our time-resolved MOBF experiment. In the first step, we subtracted a double exponential fit from the experimental data shown in Fig. 2(b) of the main manuscript. Afterward, a power spectrum (auto-correlated FFT) was applied to obtain the frequency spectrum in Figure \ref{fig:magnon}.

\begin{figure}[H]
    \centering
    \includegraphics[scale=0.4]{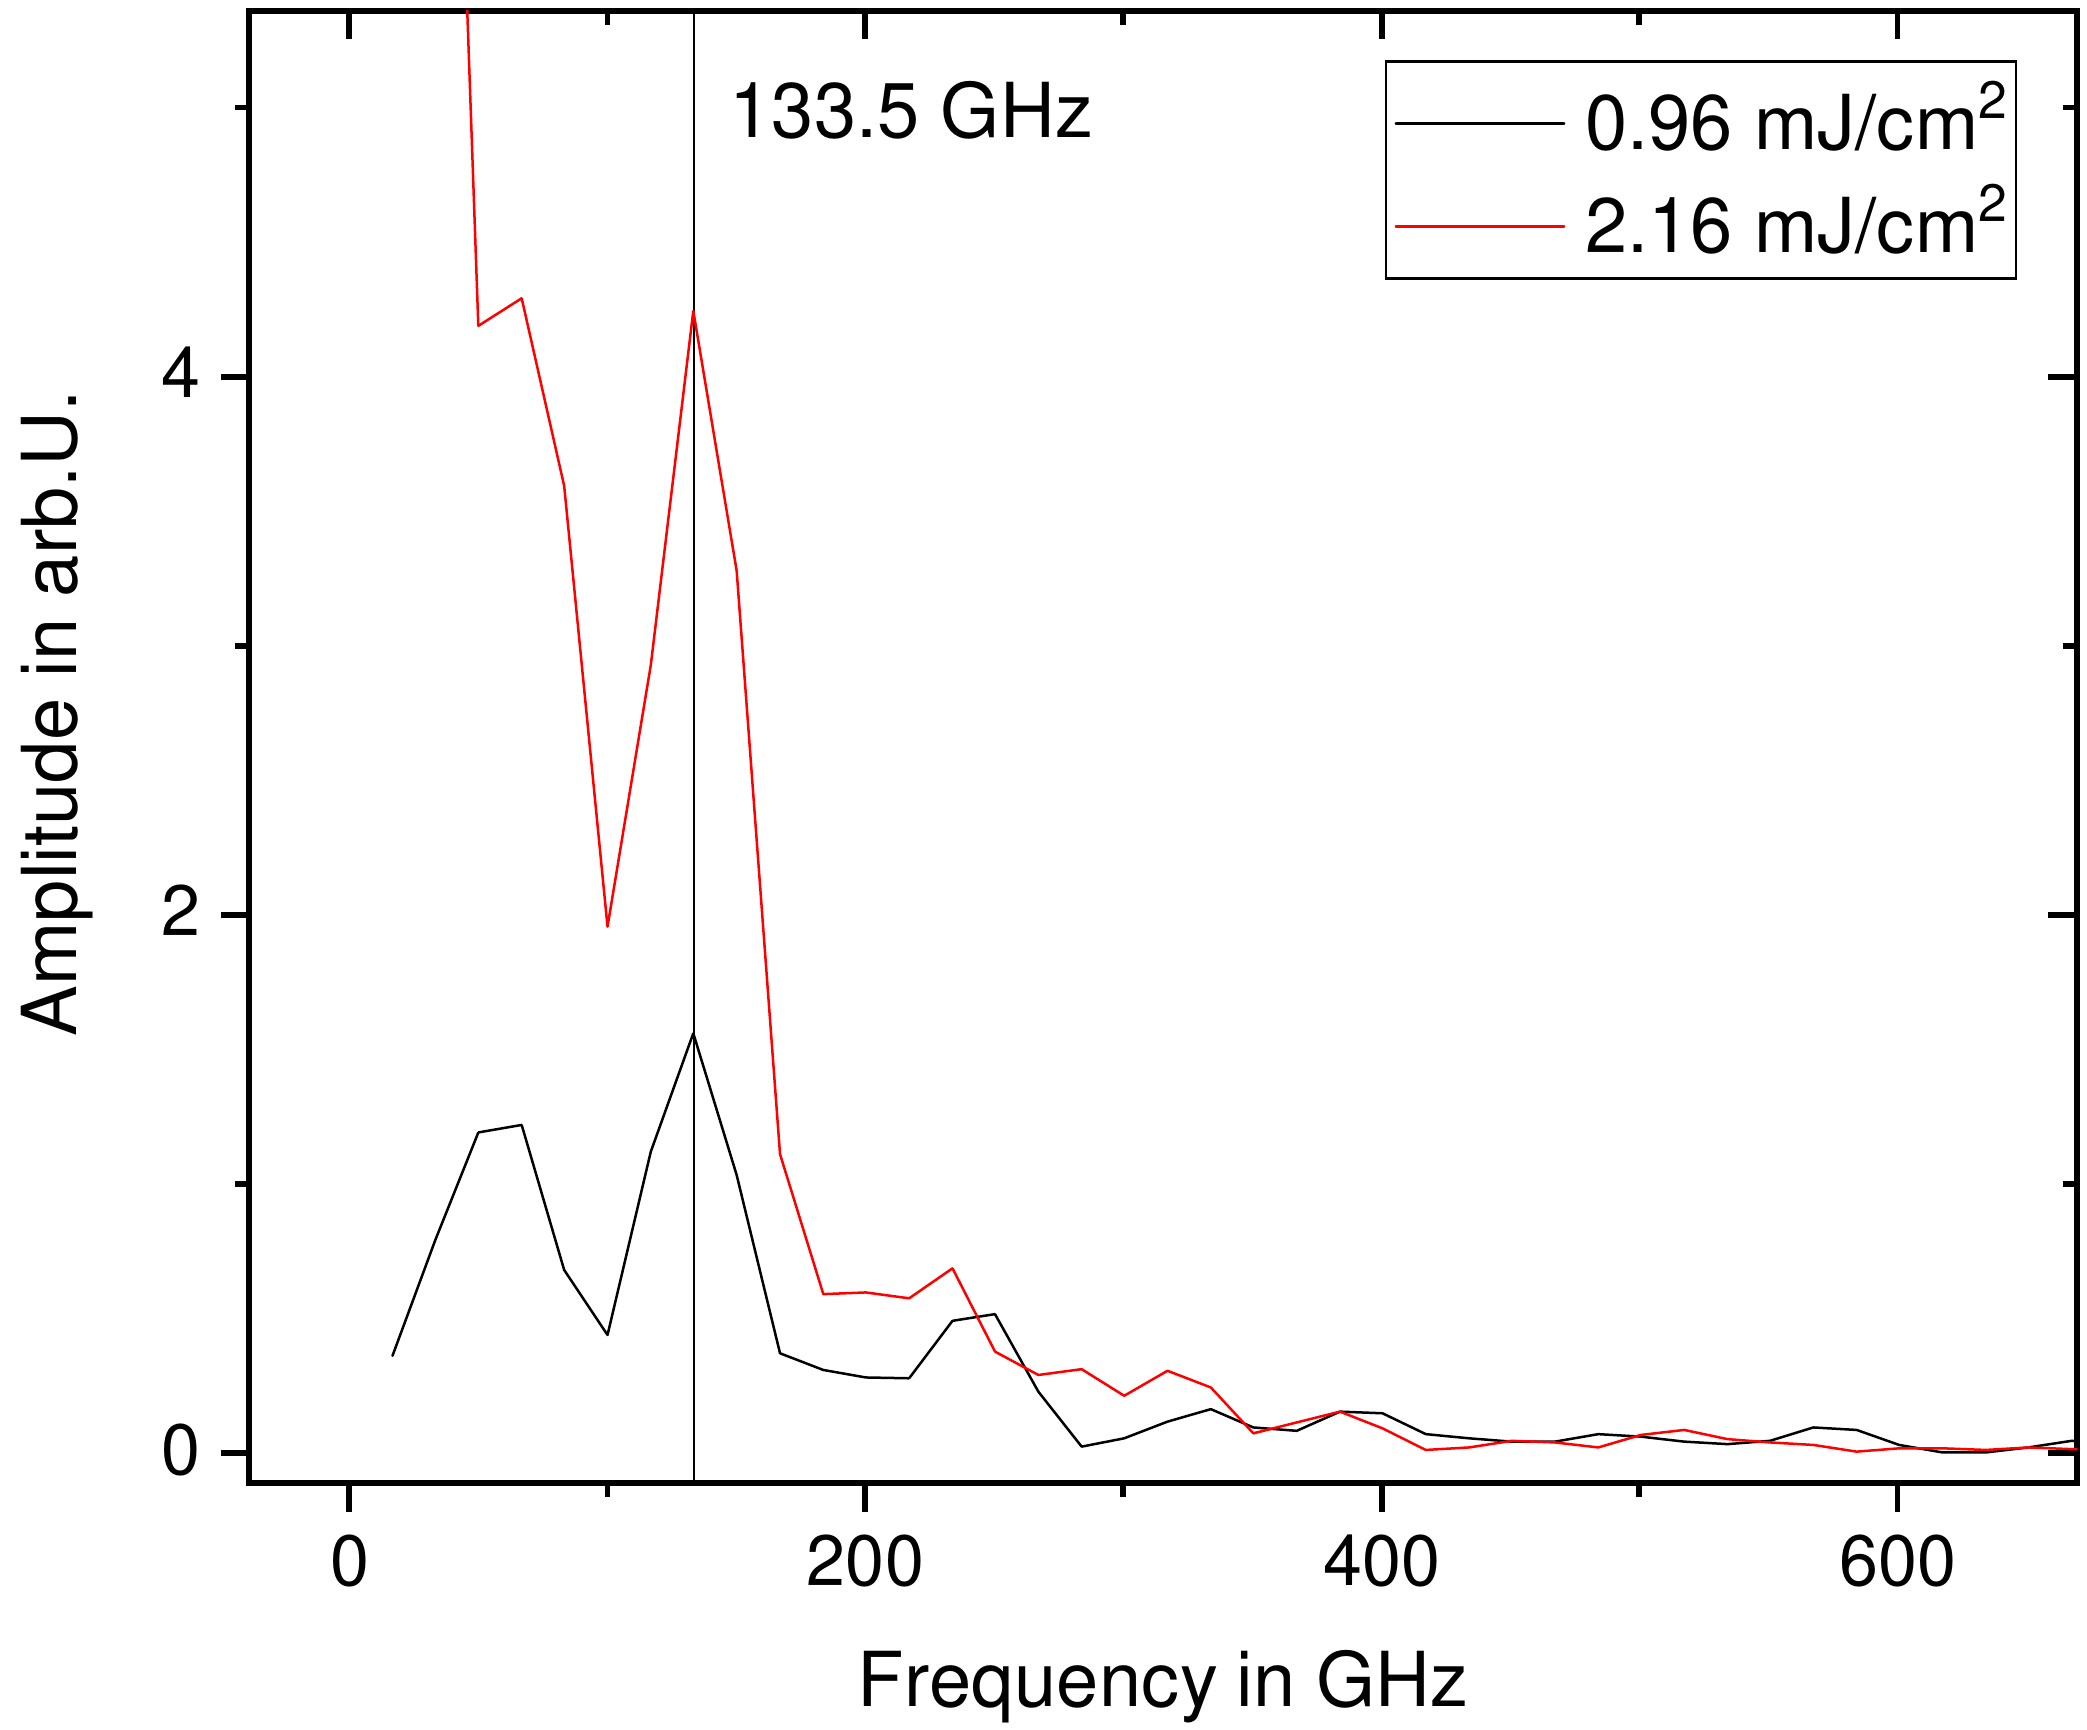}
    \caption{Power spectrum of the time-resolved MOBF traces obtained for high fluences. The marked frequency of 133.5$\,$GHz indicates the appearance of the low-frequency magnon mode in NiO.}
    \label{fig:magnon}
\end{figure}

The two extracted power spectra for the depicted fluences both show a clear peak around 133,5$\,$GHz which very much resembles reported values for the low-frequency magnon mode in NiO \cite{tzschaschel2017ultrafast, satoh2010spin, bossini2021ultrafast}

\section{Model-description of energy flow}

%We assume that the measured lattice distortion follows any temperature-induced change of the antiferromagnetic order quasi-instantaneously~\cite{Pudell2018}.

We describe the energy flow between the participating subsystems in the layers of the sample on the basis of a temperature-dependent phenomenological model. 
%
%We develop a temperature-based phenomenological model. Therefore, we assume that the measured lattice distortion follows any temperature-induced change of the antiferromagnetic order quasi-instantaneously~\cite{Pudell2018}. Furthermore, we assume homogeneous heating of the materials due to their small thicknesses.
Due to the small thicknesses of the layers, the energy within the Pt layer as well as within the NiO layer is assumed to be distributed homogeneously. %Each layer is assumed to be heated homogeneously, which is justified by their small thicknesses.
% Thereby, we explicitly exclude transport within a material and do not take into account any spatial resolution.
Therefore, transport effects within a layer can be neglected.

Similar to the two-temperature model (TTM)~\cite{Anisimov1974}, we describe the dynamics of the metallic Pt layer by electrons coupled to phonons via an electron-phonon coupling parameter $g_{ep}$. 
Its magnitude is under continuous discussion; we start with a value of 
Medvedev and Milov \cite{Medvedev2020}.
%~\cite{Anisimov1974}. 
The heat capacity of the electrons in Pt is dynamically calculated from a realistic density of stated (DOS) obtained from density functional theory (DFT)~\cite{Lin2008}, whereas for the phonons a constant heat capacity according to the Dulong-Petit law is used. 

In the insulating antiferromagnet NiO, we apply the same expression for the phononic heat capacity as in Pt. 
However, there are no free electrons in the dielectric material. 
In %the electrons are neglected, but in 
the spirit of the model proposed by \citeauthor{Beaurepaire1996} to explain their pioneering results~\cite{Beaurepaire1996}, we consider the spins a separate system. 
The coupling between spins and phonons is mediated by magneto-elastic (spin-phonon) coupling $g_{sp}$~\cite{Wall2009, Aytan2017}. 
The heat capacity of the spin system is obtained by subtracting the phononic contribution from the measured total heat capacity~\cite{Keem1978}. It exhibits a sharp peak at the Néel temperature due to the antiferromagnetic/paramagnetic phase transition and does not contribute above the Neel temperature~\cite{Radwanski2008}. 
%For heat capacity of the NiO phonons, a Debye model with a Debye temperature of $\Theta_D =\SI{650}{\kelvin}$ is used~\cite{Radwanski2008}.
%The phonons are coupled to the spins via the magneto-elastic (spin-phonon) coupling $g_{sp}$~\cite{Wall2009, Aytan2017}. 
%The energy transport across the interface between Pt and NiO could be mediated by two processes. First, energy could be transported from the Pt phonons to the NiO phonons (thin dashed line in \autoref{fig:model}~a)). However, this process is much too weak and slow to explain the ultrafast dynamics observed in the experiment, therefore it is neglected here. For the same reasons we also neglect any electron-phonon interactions across the interface, which were found to be important on ps to ns timescales~\cite{Lombard2014}. 

Possible coupling mechanisms across the Pt/NiO interface are 
electron-spin, electron-phonon and phonon-phonon coupling. 
The coupling mechanisms to the phonons act only on a pico- to nanosecond
timescale \cite{Lombard2014} and are therefore disregarded in our model. 
The electron-spin coupling can be understood as in a Pt/YIG bilayer structure \cite{seifert2018femtosecond}, where statistic scattering of 
metal electrons at the interface induce torques of the magnetic moments 
in the dielectric. 
We describe this interaction by an electron-spin coupling parameter
$\sigma_{es}$.

We further introduce an 
%During our simulations, we noticed that also the substrate has to be taken into account to accurately describe the behavior at longer timescales. It is modeled as an 
energy sink at constant temperature $T_0$ which is mediated by the phonons of the MgO substrate, draining energy from the NiO phonons. 
The rate of the energy flow is determined by the thermal boundary conductance $\sigma_{pp}$, which 
can be obtained %in principle could be calculated 
from the diffusive mismatch model (DMM)~\cite{Swartz1989}. 
All energies transported across interfaces are homogeneously distributed across the respective materials of thicknesses $d$. Then, the model reads
\begin{subequations}\label{eq:model}
\begin{align}
    \begin{split}
    c_{e,\mathrm{Pt}}\dv{T_{e,\mathrm{Pt}}}{t} %=&& \dv{u_{e,\mathrm{Pt}}}{t} 
    =& -g_{ep}(T_{e,\mathrm{Pt}} - T_{p,\mathrm{Pt}})\\
    &- \frac{\sigma_{es}}{d_\mathrm{Pt}}(T_{e,\mathrm{Pt}} - T_{s,\mathrm{NiO}}) + s(t),
    \end{split}\\
    c_{p,\mathrm{Pt}}\dv{T_{p,\mathrm{Pt}}}{t} %=&& \dv{u_{p,\mathrm{Pt}}}{t} 
    =& +g_{ep}(T_{e,\mathrm{Pt}} - T_{p,\mathrm{Pt}}), \\
    \begin{split}
    c_{s,\mathrm{NiO}}\dv{T_{s,\mathrm{NiO}}}{t} %=&& \dv{u_{s,\mathrm{NiO}}}{t} 
    =& -g_{sp}(T_{s,\mathrm{NiO}} - T_{p,\mathrm{NiO}})\\
    &+\frac{\sigma_{es}}{d_\mathrm{NiO}}(T_{e,\mathrm{Pt}} - T_{s,\mathrm{NiO}}), 
    \end{split}\\
    \begin{split}
    c_{p,\mathrm{NiO}}\dv{T_{p,\mathrm{NiO}}}{t} %=&& \dv{u_{p,\mathrm{NiO}}}{t} 
    =& +g_{sp}(T_{s,\mathrm{NiO}} - T_{p,\mathrm{NiO}}) \\
    &- \frac{\sigma_{pp}}{d_{\mathrm{NiO}}}(T_{p,\mathrm{NiO}} - T_0),
    \end{split}
\end{align}
\end{subequations}
where $s(t)$ is an energy source term accounting for the laser excitation. We apply the Crank-Nicolson scheme to solve the system of coupled differential equations (\ref{eq:model}) numerically~\cite{CrankNicolson1947}.
%\highl{Parameters?}

In our calculations, we use a Gaussian laser pulse of various fluences and \SI{50}{\femto\second} duration (FWHM) in agreement with our experiments. The four coupling parameters $g_{ep}, \sigma_{es}, g_{sp}$ and  $\sigma_{pp}$ are taken as independent on temperature. 
While the energy loss of the laser-heated Pt electrons, described with the coupling parameters $g_{ep}$ and $\sigma_{es}$, mainly influence 
the height and time of the peak of the spin temperature $T_s$,
the coupling of the spin system to the phonons in NiO is responsible for
the relaxation in the $10\,$ps range. 
The energy loss to the substrate, described by $\sigma_{pp}$, 
acts on a longer range of $\sim 100\,$ps.

We optimize these four parameters 
in comparison with the experimental MOBF trace for 
an intermediate fluence of $1.19\,$mJ cm$^2$.
Excitation with other laser fluences is simulated with the same set of parameters. 
 %constant and treated as fit parameters for our model. 

\bibliographystyle{apsrev}

\end{document}
